# Supplementary material for: Vision Transformer Neural Architecture Search for Out-of-Distribution Generalization: Benchmark and Insights
Source: arXiv:2501.03782 source file (2025-01-07)
Supplement: Supplementary file 1 [file additional_figures.tex]

\section{Main paper figures for other datasets} \label{Sec:Appx_Figures}

\subsection{Example Image of Corruptions in ImageNet-C}\label{sec:Appx_Figures_Imagenetc}

\begin{figure}[H]
	\centering
	% Use the relevant command to insert your figure file.
	% For example, with the graphicx package use
	\includegraphics[keepaspectratio,scale=0.35]{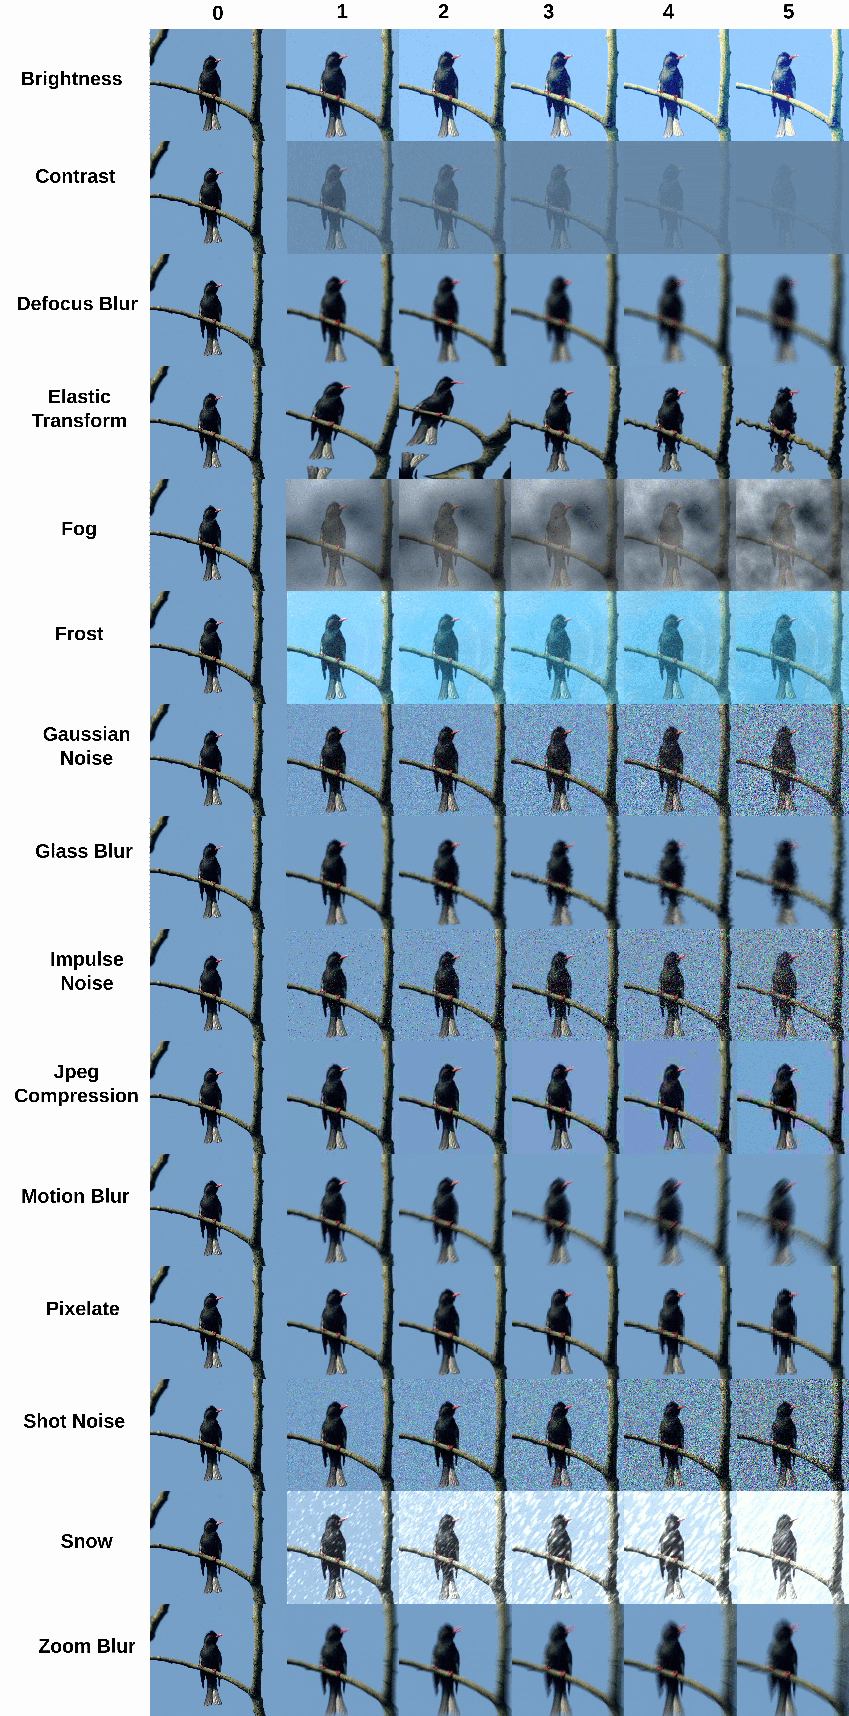}
	% figure caption is below the figure
	\caption{ An example image of IN-C (ImageNet-C) \cite{Hendrycks2018} with different corruption types at different severity levels.  }
	\label{fig:imagenet-c-example}       % Give a unique label
\end{figure}

\subsection{Visualization of OoD Accuracy Range}\label{sec:Appx_Figures_accuracy_range}

\begin{figure}[H]
	\centering
	% Use the relevant command to insert your figure file.
	% For example, with the graphicx package use
	\includegraphics[keepaspectratio,width = 14cm]{figures/violin_acc_19.png}
	% figure caption is below the figure
	\caption{Accuracy range over all unique architectures in our OoD-ViT-NAS benchmark. The numbers within each violin plot for each sub-figures (e.g., IN-C Fog 8.89(1.06), 8.00(2.25), and 5.54(0.56)) denote the corresponding OoD(ID) accuracy range of architectures sampled from AutoFormer-Tiny/Small/Base search space, respectively.}\label{fig:benchmark_accuracy_range}       % Give a unique label
\end{figure}
\subsection{ImageNet-C Common Corruption Accuracies}\label{sec:Appx_Figures_inc_accuracy}
Here, we compare the ID/OoD accuracy range of 3000 architectures with varying ViT architectures to capture a different aspect of robustness generalization. \somayeh{include 5 levels of corruption violin plot}

\subsection{ImageNet-P Accuracies}\label{sec:Appx_Figures_inp_accuracy}

\subsection{Effect of ViT Architectural Design on OoD Robustness}\label{Sec:Appx_Figures_Embedding}

\subsubsection{Additional correlation analysis }\label{Sec:Appx_Arch_Correlation}

\somayeh{we will include detailed dataset correlation and proxy correlation for each supernet}
\subsubsection{Effect of embedding dimension on OoD generalization }\label{Sec:Appx_Figures_Embedding}

In our ablation study, we look at the correlation between embedding dimension and ID/OoD accuracy. We fix the network depth at 13 layers while varying the embedding dimension. The result is shown in Figure \ref{fig:ablation-edim}. We find an overall positive correlation of 0.627, suggesting that the embedding dimension can be a good indicator of the model's robustness. For example, higher embedding dimensions improve performance in synthetic corruption of IN-C but are less effective for synthetic images generated in the IN-D dataset, where the correlation becomes close to zero or even negative (as shown in Figure \ref{fig:embedding} and \ref{fig:ablation-edim}).

\begin{figure}[!ht]
	\centering
	% Use the relevant command to insert your figure file.
	% For example, with the graphicx package use
	\includegraphics[keepaspectratio,scale=0.40]{figures/id_ood_arch_heatmap_small_embed.png}
	% figure caption is below the figure

	\caption{Ablation study on different embedding dimensions on ID/OoD generalization. Kendall rank correlation coefficient between ID/OoD accuracies and embedding dimension for 325 architectures with 13-layer depth. This plot shows a positive correlation between Embed\_Dim and ID/OoD accuracies for most OOD shift datasets, whereas, for IN-D, the correlation becomes close to zero or even negative.  }
	\label{fig:ablation-edim}       % Give a unique label
\end{figure} 

\begin{figure}[!htb]
	\centering
	% Use the relevant command to insert your figure file.
	% For example, with the graphicx package use
	\includegraphics[keepaspectratio,scale=0.30]{figures/embedding_dim/id_ood_embedding_small_27.png}
	% figure caption is below the figure
	\caption{As in Figure \ref{fig:embedding}, we show that higher ID/OoD accuracy can be obtained by increasing the embedding dimension of architectures sampled from \textbf{AutoFormer-Small}. Our observation shows that increasing the network depth does not have a high impact on OoD robustness.   }
	\label{fig:embedding-all-small}       % Give a unique label
\end{figure}

%\begin{figure}[htb!]
%	\centering
%	% Use the relevant command to insert your figure file.
%	% For example, with the graphicx package use
%	\includegraphics[keepaspectratio,scale=0.30]{figures/embedding_dim/id_ood_embedding_small_14.png}
%	% figure caption is below the figure
%	\caption{As in Figure \ref{fig:embedding}, we show that higher ID/OoD accuracy can be obtained by increasing the embedding dimension of ViT blocks. Our observation shows that increasing the network depth does not have a high impact on OoD robustness.   }
%	\label{fig:embedding-all}       % Give a unique label
%\end{figure}

\begin{figure}[!htb]
	\centering
	% Use the relevant command to insert your figure file.
	% For example, with the graphicx package use
	\includegraphics[keepaspectratio,scale=0.30]{figures/embedding_dim/id_ood_embedding_base_all.png}
	% figure caption is below the figure
	\caption{The effect of \#Embed\_Dim on robustness generalization of 1000 architectures sampled from \textbf{AutoFormer-Base}.} % we show that higher ID/OoD accuracy can be obtained by increasing the embedding dimension of ViT blocks. Our observation shows that increasing the network depth does not have a high impact on OoD robustness.   }
	\label{fig:embedding-all-base}       % Give a unique label
\end{figure}

\begin{figure}[!htb]
	\centering
	% Use the relevant command to insert your figure file.
	% For example, with the graphicx package use
	\includegraphics[keepaspectratio,scale=0.30]{figures/embedding_dim/id_ood_embedding_tiny_all.png}
	% figure caption is below the figure
	\caption{The effect of \#Embed\_Dim on robustness generalization of 1000 architectures sampled from \textbf{AutoFormer-Tiny}. }% we show that higher ID/OoD accuracy can be obtained by increasing the embedding dimension of ViT blocks. Our observation shows that increasing the network depth does not have a high impact on OoD robustness.   }
	\label{fig:embedding-all-tiny}       % Give a unique label
\end{figure}

\subsubsection{Effect of Depth}\label{Sec:Appx_Figures_Depth}

Based on Figure \ref{fig:embedding}, for a given embedding dimension (represented by a distinct color), we report the mean accuracy, showing how the mean OoD accuracy changes among ViT architectures of varying depths. We observe that \textit{increasing the network depth does not significantly improve OOD generalization of the architectures in our benchmark}, which aligns with the observations in \cite{Levine2020}. In particular, we observe that ID accuracy with an average-accuracy range of 1.22\% does not change much across all architectures with various numbers of layers (Figure \ref{fig:embedding}, left panel). There, as shown in Figure \ref{fig:embedding-all-small} in Appendix \ref{Sec:Appx_Figures_Embedding}, the average-accuracy range (1.99\%) on our robustness benchmarks is boosted by less than 0.77\%, while the span of mean OoD accuracies remains large, ranging from 0.44\% to 5.86\%. Meanwhile, our analysis also confirms that increasing the depth is not very effective in improving the OoD performance for models sampled from Tiny and Base supernets as well, where the mean OoD accuracies of these networks range in $[0.01,0.92]$ and $[0.05,1.05]$, respectively (see Figure \ref{fig:embedding-all-tiny} and \ref{fig:embedding-all-base}). This indicates that deeper models might not always be beneficial, especially when handling certain OoD distribution shifts. 
% TODO

Figure \ref{fig:depth} depicts the ranking correlation for all architectures between depth and ID/OoD accuracies. In our ablation study, we analyze how variations in the depth parameter affect the model’s robustness by maintaining those architectures with a certain embedding dimension (e.g., Embed\_Dim $=384$). Our analysis shows that increasing the depth can be relatively correlated with high ID accuracy in subnets derived from AutoFormer-Small; however, this increase in depth might not necessarily translate into the OoD distribution shifts and model robustness. This plot shows a positive correlation between the depth for IN-P, IN-R, and IN-A OoD shift, whereas, for all other distribution shifts, the correlation becomes close to zero or even negative. Overall, our findings suggest that increasing network depth significantly narrows the gap between ID and OoD accuracies, indicating that network depth contributes little to OoD robustness in our benchmarks. Further details can be found in Appendix \ref{Sec:Appx_Arch_Correlation}.

%The average OoD classification accuracy results in each depth in Figure \ref{fig:embedding-all-small} (Appendix \ref{appendixB}) also confirm the insignificant effectiveness of depth. Moreover, increasing the network depth 

\begin{figure}[!htb]
	\centering
	% Use the relevant command to insert your figure file.
	% For example, with the graphicx package use
	\includegraphics[keepaspectratio,scale=0.40]{figures/id_ood_arch_heatmap_small_depth.png}
	% figure caption is below the figure
	\caption{Kendall rank correlation coefficient between the network depth and all OoD robust accuracies evaluated on 308 architectures with Embed\_Dim $=384$ and varying depths. The correlation of ranking at bottom is the continuation of rank table of other OoD shifts at the top. }
	\label{fig:depth}       % Give a unique label
\end{figure}

\subsubsection{Effect of MLP Ratio on OoD Generalization }\label{Sec:Appx_Figures_Mlp}

The MLP ratio (or expansion ratio) expands the input embedding dimension by a factor at each layer. To investigate how varying the MLP ratio at each layer affects OoD robustness, we design the layer-wise analysis to investigate the influence of the MLP ratio in each layer by changing the MLP ratio in each layer for our ablation study. 

In AutoFormer-Small search space, the MLP ratio at any given layer — referred to as the $i$-th layer — can be set to 3, 3.5, or 4. We construct a dataset consisting of robust accuracies of 108 randomly sampled from AutoFormer-Small, where the sampled models are fixed with three architectural design components: (Depth = 12, Embed\_Dim = 320, \#Heads = 5). With these parameters fixed, the total number of potential MLP ratio configurations is extensive (i.e., $3^{12}$), making it impractical to evaluate every possible configuration for analysis. Therefore, to specifically assess the influence of the MLP ratio at the $i$-th layer, we maintained a constant MLP ratio across all other layers and then measured the OoD robust accuracies.  Figure \ref{fig:mlp-configuration} in Appendix \ref{Sec:Appx_Figures_Mlp} shows the possible nine configurations of MLP ratio at $5$-th layer. In Table \ref{tab:ablation-mlp}, we observe that changing the MLP ratio at layers \#4 and \#5 leads to an increased range of mean OoD robust accuracy. %Further details can be found in Appendix \ref{Sec:Appx_Figures_Mlp}. 

\input{tables/ablation-mlp.tex} 

\begin{figure}[!htb]
	\centering
	% Use the relevant command to insert your figure file.
	% For example, with the graphicx package use
	\includegraphics[keepaspectratio,scale=0.5]{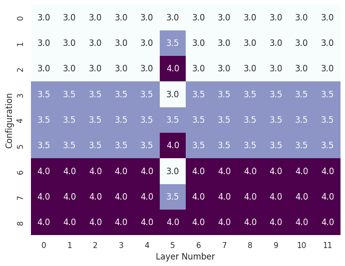}
	% figure caption is below the figure
	\caption{The possible configurations of MLP ratio at $5$-th layer of 108 architectures sampled from \textit{AutoFormer-Small} in ablation study. }% we show that higher ID/OoD accuracy can be obtained by increasing the embedding dimension of ViT blocks. Our observation shows that increasing the network depth does not have a high impact on OoD robustness.   }
\label{fig:mlp-configuration}       % Give a unique label
\end{figure}

\begin{figure}[!htb]
	\centering
	% Use the relevant command to insert your figure file.
	% For example, with the graphicx package use
	\includegraphics[keepaspectratio,scale=0.35]{figures/mlp/OOD Acc IN-C Fog 5_all_layers_3.0.png}
	% figure caption is below the figure
	\caption{	A visualization on the effect of changing MLP Ratio per layer to OoD Accuracy in 108 architectures sampled from \textit{AutoFormer-Small} in ablation study. To evaluate the effect of layer $i$-th, we fix the MLP ratio $=3.0$ for the remaining layers. We observe that higher OoD accuracy range can be obtained by changing the MLP ratio at layer 4 and 5. 
	}% we show that higher ID/OoD accuracy can be obtained by increasing the embedding dimension of ViT blocks. Our observation shows that increasing the network depth does not have a high impact on OoD robustness.   }
\label{fig:mlp-configuration1}       % Give a unique label
\end{figure}

\begin{figure}[!htb]
	\centering
	% Use the relevant command to insert your figure file.
	% For example, with the graphicx package use
	\includegraphics[keepaspectratio,scale=0.35]{figures/mlp/OOD Acc IN-C Fog 5_all_layers_3.5.png}
	% figure caption is below the figure
	\caption{A visualization on the effect of changing MLP Ratio per layer to OoD Accuracy in 108 architectures sampled from \textit{AutoFormer-Small} in ablation study. To evaluate the effect of layer $i$-th, we fix the MLP ratio $=3.5$ for the remaining layers.  We observe that higher OoD accuracy range can be obtained by changing the MLP ratio at layer 4 and 5. }% we show that higher ID/OoD accuracy can be obtained by increasing the embedding dimension of ViT blocks. Our observation shows that increasing the network depth does not have a high impact on OoD robustness.   }
\label{fig:mlp-configuration2}       % Give a unique label
\end{figure}

\begin{figure}[!htb]
	\centering
	% Use the relevant command to insert your figure file.
	% For example, with the graphicx package use
	\includegraphics[keepaspectratio,scale=0.35]{figures/mlp/OOD Acc IN-C Fog 5_all_layers_4.0.png}
	% figure caption is below the figure
	\caption{A visualization on the effect of changing MLP Ratio per layer to OoD Accuracy in 108 architectures sampled from \textit{AutoFormer-Small} in ablation study. To evaluate the effect of layer $i$-th, we fix the MLP ratio $=4.0$ for the remaining layers. We observe that a higher OoD accuracy range can be obtained by changing the MLP ratio at layers 4 and 5. }% we show that higher ID/OoD accuracy can be obtained by increasing the embedding dimension of ViT blocks. Our observation shows that increasing the network depth does not have a high impact on OoD robustness.   }
\label{fig:mlp-configuration3}       % Give a unique label
\end{figure}
